# Supplementary material for: Atomic photoionization cross-sections beyond the electric dipole approximation
Source: arXiv:1810.08542 source file (2018-10-19)
Supplement: Supplementary file 1 [file SupplementaryMaterial.pdf]

# Supplementary Material: Atomic photoionization cross-sections beyond the electric dipole approximation

Iulia Emilia Brumboiu,[1,2,a] Olle Eriksson,[3] and Patrick Norman[1]

[1] *Department of Theoretical Chemistry and Biology, KTH Royal Institute of Technology, 10691 Stockholm, Sweden*

[2] *Department of Chemistry, Korea Advanced Institute for Science and Technology, 34141 Daejeon, Korea*

[3] *Department of Physics and Astronomy, Uppsala University, 75120 Uppsala, Sweden*

The following are provided below: **a)** the derivation of the linear response function to a time-dependent perturbation $\hat{V}(t)$ for a generic operator $\hat{O}$; **b)** analytical formulas for the transition matrix elements involving Gaussian type orbitals and plane waves; **c)** photoionization cross-sections calculated using different basis sets for N; **d)** the analytical form of a transition matrix element between a simplified 2s orbital (described as a linear combination of two GTOs) and a plane wave.

[a] iubr@kth.se

## LINEAR RESPONSE FUNCTION FOR A GENERIC OPERATOR

We start from the expression of the interaction Hamiltonian:

$$\hat{H}(t) = \hat{H}_0 + \sum_{\omega_2=\pm\omega} \hat{V}^{\omega_2} e^{-i\omega_2 t} \tag{S1}$$

where $\hat{H}_0$ is the unperturbed time-independent Hamiltonian and we have chosen the name $\omega_2$ for the summation variable in order to be be consistent with the notation used in the main text. Before the perturbation is turned on, we assume the system is in its electronic ground state:

$$\hat{H}_0 |0\rangle = E_0 |0\rangle \tag{S2}$$

The excited states of the same Hamiltonian are denoted $\{|n\rangle\}$ with the corresponding eigenvalues $\{E_n\}$:

$$\hat{H}_0 |n\rangle = E_n |n\rangle \,, \;\; n > 0 \tag{S3}$$

The time-dependent state $|0(t)\rangle$ may be expressed in terms of a unitary transformation of the time-independent ground state $|0\rangle$:[1]

$$|0(t)\rangle = e^{i\hat{P}(t)/\hbar} |0\rangle \tag{S4}$$

where the Hermitian operator $\hat{P}(t)$ is expressed as:

$$\hat{P}(t) = \sum_{n>0} \left[P_n(t)\Lambda_n + P_n^*(t)\Lambda_{-n}\right] \tag{S5}$$

$$\Lambda_n = |n\rangle \langle 0| \tag{S6}$$

$$\Lambda_{-n} = |0\rangle \langle n| \tag{S7}$$

$P_n(t)$ are complex time-dependent state-transfer amplitudes which may be expanded in series in terms of the perturbation $\hat{V}(t)$:

$$P_n(t) = P_n^{(0)}(t) + P_n^{(1)}(t) + P_n^{(2)}(t) + ... \tag{S8}$$

which corresponds to an expansion of the time-dependent state $|0(t)\rangle$:

$$|0(t)\rangle = |0^{(0)}\rangle + |0^{(1)}\rangle + |0^{(2)}\rangle + ... \tag{S9}$$

By inserting Eq. (S8) into Eq. (S4) and considering that $P_n^0$ vanishes because $|0\rangle$ is an eigenstate of the unperturbed Hamiltonian,[1] the terms of the same order are identified. Specifically, the

first three terms are:

$$|0^{(0)}\rangle = |0\rangle \tag{S10}$$

$$|0^{(1)}\rangle = \frac{i}{\hbar}\sum_{n>0} P_n^{(1)}(t)\,|n\rangle \tag{S11}$$

$$|0^{(2)}\rangle = \frac{i}{\hbar}\sum_{n>0} P_n^{(2)}(t)\,|n\rangle - \frac{1}{2\hbar^2}\sum_{n>0} P_n^{(1)}(t)P_n^{*(1)}(t)\,|0\rangle \tag{S12}$$

To obtain differential equations for the first order amplitudes $P_k^{(1)}(t)$, we use the Ehrenfest theorem for the operators $\Lambda_k$ and $\Lambda_{-k}$:[1]

$$\langle 0(t)|\,\Lambda_k\,|\dot{0}(t)\rangle + \langle \dot{0}(t)|\,\Lambda_k\,|0(t)\rangle = -\frac{i}{\hbar}\,\langle 0(t)|\,[\Lambda_k, \hat{H}_0 + \hat{V}(t)]\,|0(t)\rangle \tag{S13}$$

$$\langle 0(t)|\,\Lambda_{-k}\,|\dot{0}(t)\rangle + \langle \dot{0}(t)|\,\Lambda_{-k}\,|0(t)\rangle = -\frac{i}{\hbar}\,\langle 0(t)|\,[\Lambda_{-k}, \hat{H}_0 + \hat{V}(t)]\,|0(t)\rangle \tag{S14}$$

By replacing $|0(t)\rangle$ in Eq. S13 with the series expansion from Eq. (S9) and by retaining only the first order terms, we obtain:

$$\langle 0|\,\Lambda_k\,|\dot{0}^{(1)}\rangle + \langle \dot{0}^{(1)}|\,\Lambda_k\,|0\rangle + \frac{i}{\hbar}\,\langle 0|\,[\Lambda_k, \hat{H}_0]\,|0^{(1)}\rangle + \frac{i}{\hbar}\,\langle 0^{(1)}|\,[\Lambda_k, \hat{H}_0]\,|0\rangle = -\frac{i}{\hbar}\,\langle 0|\,[\Lambda_k, \hat{V}(t)]\,|0\rangle \tag{S15}$$

By further using Eq. (S11) to express $|0^{(1)}\rangle$ and applying Eqs. (S2) and (S3), we obtain:

$$\sum_{n>0}\left(i\dot{P}_n^{(1)}(t)\,\langle 0|\,\Lambda_k\,|n\rangle - i\dot{P}_n^{*(1)}(t)\,\langle n|\,\Lambda_k\,|0\rangle - \frac{E_n - E_0}{\hbar}P_n^{(1)}(t)\,\langle 0|\,\Lambda_k\,|n\rangle - \frac{E_n - E_0}{\hbar}P_n^{*(1)}(t)\,\langle n|\,\Lambda_k\,|0\rangle\right)$$
$$= -i\,\langle 0|\,[\Lambda_k, \hat{V}(t)]\,|0\rangle \tag{S16}$$

A similar expression for $\Lambda_{-k}$ is obtained by the same procedure, but starting from Eq. (S14). Finally, using the explicit definitions of $\Lambda_k$ and $\Lambda_{-k}$ from Eqs. (S6) and (S7), we obtain the following differential equations for the first order state-transfer amplitudes:

$$i\dot{P}_k^{(1)}(t) - \frac{(E_k - E_0)}{\hbar}P_k^{(1)}(t) = -i\,\langle k|\,\hat{V}(t)\,|0\rangle \tag{S17}$$

$$-i\dot{P}_k^{*(1)}(t) - \frac{(E_k - E_0)}{\hbar}P_k^{*(1)}(t) = i\,\langle 0|\,\hat{V}(t)\,|k\rangle \tag{S18}$$

The solutions of these equations are of the type:

$$P_k^{(1)}(t) = -e^{-i\omega_{k0}t}\int_0^t e^{i\omega_{k0}\tau}\,\langle k|\,\hat{V}(\tau)\,|0\rangle\;\mathrm{d}\tau \tag{S19}$$

$$P_k^{*(1)}(t) = -e^{i\omega_{k0}t}\int_0^t e^{-i\omega_{k0}\tau}\,\langle 0|\,\hat{V}(\tau)\,|k\rangle\;\mathrm{d}\tau \tag{S20}$$

with $\omega_{k0} = (E_k - E_0)/\hbar$ and where we have considered the perturbation is turned on at time $t_0 = 0$. Differential equations for the second-order, third-order and higher order terms may be

found in a similar way.

Replacing the time-dependent interaction potential with its expression in Eq. S1, we obtain:

$$P_k^{(1)}(t) = -e^{-i\omega_{k0}t} \sum_{\omega_2=\pm\omega} \langle k| \hat{V}^{\omega_2} |0\rangle \int e^{i(\omega_{k0}-\omega_2)\tau}\, \mathrm{d}\tau = \sum_{\omega_2=\pm\omega} \frac{ie^{-i\omega_2 t}}{\omega_{k0}-\omega_2-i\gamma_k} \langle k| \hat{V}^{\omega_2} |0\rangle \quad \text{(S21)}$$

$$P_k^{*(1)}(t) = -e^{i\omega_{k0}t} \sum_{\omega_2=\pm\omega} \langle 0| \hat{V}^{\omega_2} |k\rangle \int e^{-i(\omega_{k0}+\omega_2)\tau}\, \mathrm{d}\tau = \sum_{\omega_2=\pm\omega} \frac{-ie^{-i\omega_2 t}}{\omega_{k0}+\omega_2+i\gamma_k} \langle 0| \hat{V}^{\omega_2} |k\rangle \quad \text{(S22)}$$

where $\gamma_k$ is the half-width broadening associated with the lifetime of the excited state.

The time development of the average value of an operator $\hat{O}$ can be calculated using $|0(t)\rangle$:

$$\left\langle \hat{O} \right\rangle_t = \langle 0(t)| \hat{O} |0(t)\rangle \quad \text{(S23)}$$

At the same time, the average value of $\hat{O}$ may be formally expanded as:[1,2]

$$\left\langle \hat{O} \right\rangle_t = \langle 0| \hat{O} |0\rangle + \hat{V}(t) \left\langle\left\langle \hat{O}; \hat{V}^{\pm\omega} \right\rangle\right\rangle + \frac{1}{2}\hat{V}^2(t) \left\langle\left\langle \hat{O}; \hat{V}^{\pm\omega}, \hat{V}^{\pm\omega} \right\rangle\right\rangle + ... \quad \text{(S24)}$$

where $\left\langle\left\langle \hat{O}; \hat{V}^{\pm\omega} \right\rangle\right\rangle$ denotes the linear response function, $\left\langle\left\langle \hat{O}; \hat{V}^{\pm\omega}, \hat{V}^{\pm\omega} \right\rangle\right\rangle$ denotes the quadratic response function, and so on.

Replacing $0(t)$ in Eq. (S23) with the expansion from Eq. (S9) and identifying the terms which are linear, quadratic, cubic, etc. in the perturbation, the corresponding response functions may be determined explicitly. The linear response function which is of interest for us is obtained by identifying the terms which are linear in $\hat{V}(t)$:

$$\hat{V}(t) \left\langle\left\langle \hat{O}; \hat{V}^{\pm\omega} \right\rangle\right\rangle = \langle 0| \hat{O} |0^{(1)}\rangle + \langle 0^{(1)}| \hat{O} |0\rangle \quad \text{(S25)}$$

Finally, the linear response function is:

$$\left\langle\left\langle \hat{O}; \hat{V}^{\pm\omega} \right\rangle\right\rangle = -\frac{1}{\hbar} \sum_{n>0} \sum_{\omega_2=\pm\omega} \left( \frac{\langle 0| \hat{O} |n\rangle \langle n| \hat{V}^{\omega_2} |0\rangle}{\omega_{n0}-\omega_2-i\gamma_n} + \frac{\langle n| \hat{O} |0\rangle \langle 0| \hat{V}^{\omega_2} |n\rangle}{\omega_{n0}+\omega_2+i\gamma_n} \right) \quad \text{(S26)}$$

## ANALYTICAL FORMULAS FOR THE TRANSITION MATRIX ELEMENTS

The transition matrix element we are after is:

$$\langle g_{lx,ly,lz}|e^{i\mathbf{k}_\mathrm{e}\cdot\mathbf{r}-i\mathbf{k}\cdot\mathbf{r}}\rangle = \int\limits_{-\infty}^{\infty}\int\limits_{-\infty}^{\infty}\int\limits_{-\infty}^{\infty} g_{lx,ly,lz}(x,y,z)e^{i\mathbf{K}\cdot\mathbf{r}}\,\mathrm{d}x\,\mathrm{d}y\,\mathrm{d}z, \quad \text{(S27)}$$

where $g_{l_x,l_y,l_z}$ is a normalized Gaussian primitive, $l = l_x + l_y + l_z$:[3]

$$g_{l_x,l_y,l_z} = N_{l_xl_yl_z}(x-R_x)^{l_x}(y-R_y)^{l_y}(z-R_z)^{l_z}e^{-\alpha\left[(x-R_x)^2+(y-R_y)^2+(z-R_z)^2\right]}, \quad \text{(S28)}$$
$$N_{l_xl_yl_z} = \left(\frac{2\alpha}{\pi}\right)^{3/4}\left[\frac{(8\alpha)^l\,l_x!\,l_y!\,l_z!}{(2l_x)!\,(2l_y)!\,(2l_z)!}\right],$$

$\mathbf{K}\cdot\mathbf{r} = Kx + Ky + Kz$, with $\mathbf{K}$ determined from the photon wavevector $\mathbf{k}$ (input parameter) and the photoelectron wavevector $\mathbf{k}_\mathrm{e}$ (determined from energy conservation).
By separating the triple integral into components, the matrix element becomes:

$$\langle g_{lx,ly,lz}|e^{i\mathbf{K}\cdot\mathbf{r}}\rangle = N_{l_xl_yl_z}I_xI_yI_z \quad \text{(S29)}$$

with $I_w$ (where $w = x,\ y,\ z$) is an integral of the type:

$$I_w = \int\limits_{-\infty}^{\infty}(w-R_w)^{l_w}e^{-\alpha(w-R_w)^2+iwK_w}\,\mathrm{d}w \quad \text{(S30)}$$

Making the change of variable $v = w - R_w$, $I_w$ becomes:

$$I_w = e^{iK_wR_w}\int\limits_{-\infty}^{\infty}v^{l_w}e^{-\alpha v^2+ivK_w}\,\mathrm{d}v \quad \text{(S31)}$$

Analytical formulas for the integral over $v$ may be obtained iteratively, starting with $l_w = 0$, and by differentiating with respect to $K_w$, as described in detail in Ref. [4]. We have used this

algorithm to obtain formulas up to $l_w = 5$, which we provide below:

$$I_0 = \int_{-\infty}^{\infty} e^{-\alpha v^2 + ivK_w}\,\mathrm{d}v = \sqrt{\frac{\pi}{\alpha}}\,e^{-K_w^2/(4\alpha)} \tag{S32}$$

$$I_1 = \int_{-\infty}^{\infty} v\,e^{-\alpha v^2 + ivK_w}\,\mathrm{d}v = \frac{iK_w}{2\alpha}\,I_0 \tag{S33}$$

$$I_2 = \int_{-\infty}^{\infty} v^2 e^{-\alpha v^2 + ivK_w}\,\mathrm{d}v = \frac{1}{2\alpha}\left(1 - \frac{K_w^2}{2\alpha}\right) I_0 \tag{S34}$$

$$I_3 = \int_{-\infty}^{\infty} v^3 e^{-\alpha v^2 + ivK_w}\,\mathrm{d}v = \frac{iK_w}{4\alpha^2}\left(3 - \frac{K_w^2}{2\alpha}\right) I_0 \tag{S35}$$

$$I_4 = \int_{-\infty}^{\infty} v^4 e^{-\alpha v^2 + ivK_w}\,\mathrm{d}v = \frac{1}{4\alpha^2}\left(3 - \frac{3K_w^2}{\alpha} + \frac{K_w^4}{4\alpha^2}\right) I_0 \tag{S36}$$

$$I_5 = \int_{-\infty}^{\infty} v^5 e^{-\alpha v^2 + ivK_w}\,\mathrm{d}v = \frac{iK_w}{8\alpha^3}\left(15 - \frac{5K_w^2}{\alpha} + \frac{K_w^4}{4\alpha^2}\right) I_0 \tag{S37}$$

## BASIS SET DATA FOR THE NITROGEN ATOM

Partial photoionization cross-sections for the 2s and 2p orbitals of the N atom, computed with six different basis sets are shown in the figure below. The figure shows that the 2p cross-

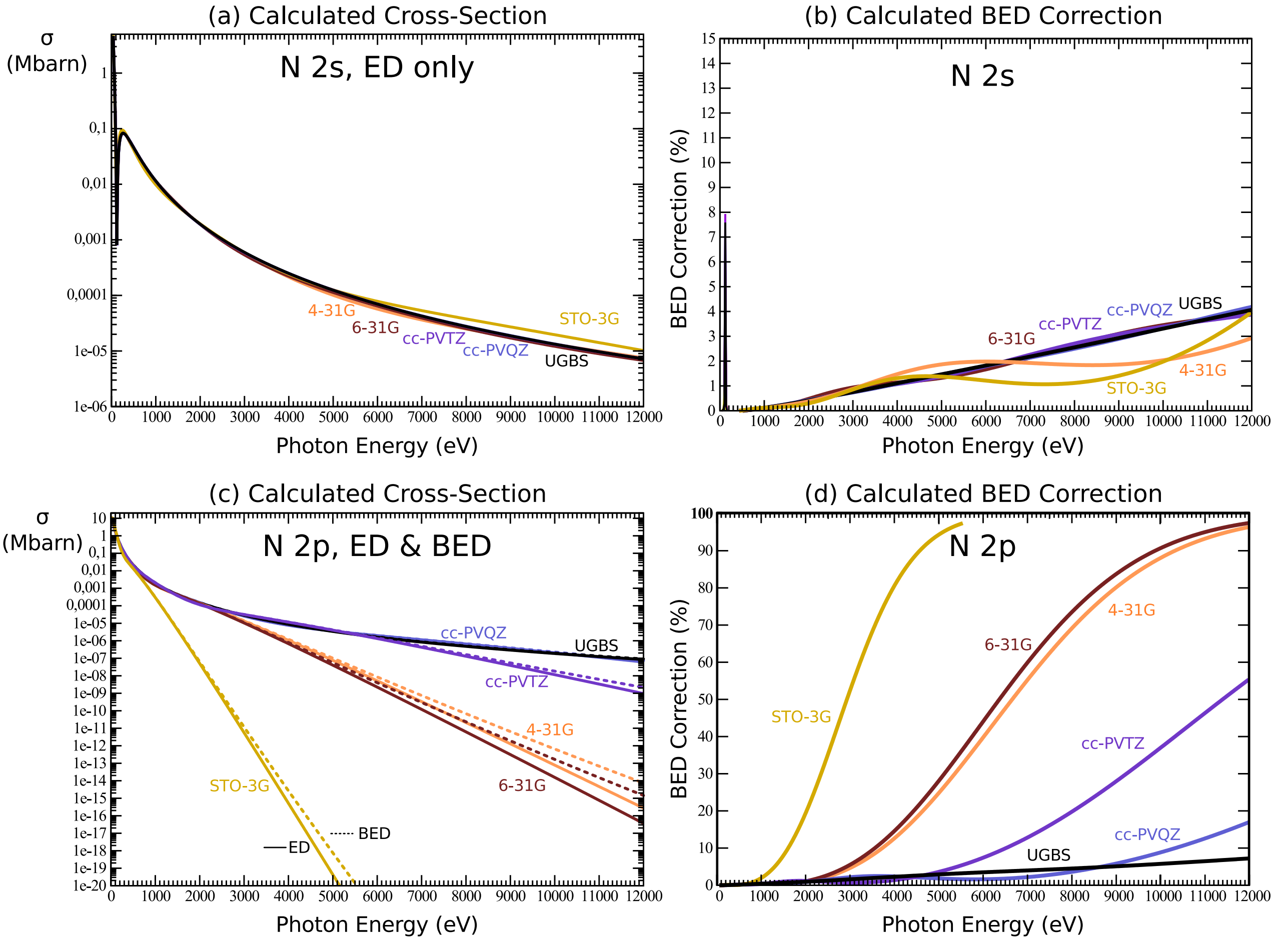


Figure S1. Calculated photoionization cross-sections and BED corrections for the 2s (a,b) and 2p (c,d) orbitals of the N atom. The calculations were performed using different basis sets, namely STO-3G (yellow), 4-31G (orange), 6-31G (red), cc-pVTZ (purple), cc-pVQZ (blue) and UGBS (black). For clarity, in (a) only the dipole cross-sections are shown because the BED values are almost indistinguishable. (Note that the cross-sections have **not** been multiplied by the 1/3 factor, as was performed in the main text.)

.

sections are particularly sensitive to the choice of basis set, the results appearing to converge once a large and accurate enough basis is selected. We have, therefore, opted to perform all calculations reported in the main text with the UGBS basis set, which also results in a linearly increasing BED correction (as opposed to a non-linear increase when smaller basis sets are used, especially evident in Fig. S1b).

## TRANSITION MATRIX ELEMENT FOR A SIMPLIFIED 2S ORBITAL

Assume a simplified form of a 2s atomic orbital, centred at the origin and represented as a linear combination of two Gaussian type orbitals (GTOs):

$$\chi_{\mathrm{GTO}} = c_1 e^{-\alpha_1(x^2+y^2+z^2)} + c_2 e^{-\alpha_2(x^2+y^2+z^2)}, \tag{S38}$$

where $c_1 < 0$, $c_2 > 0$, and $\alpha_1, \alpha_2 > 0$, and the normalization constant has been left out for simplicity. We further assume that upon ionization, the photoelectron can be described by a plane wave with wavevector $k_{\mathrm{e}}$ pointing in the z-direction:

$$\chi_f = e^{ik_{\mathrm{e}}z}. \tag{S39}$$

Within the dipole approximation, the photoionization cross-section involves transition matrix elements of the type:

$$\begin{aligned}
\langle \chi_{\mathrm{GTO}} | \chi_f \rangle &= \langle c_1 e^{-\alpha_1(x^2+y^2+z^2)} + c_2 e^{-\alpha_2(x^2+y^2+z^2)} | e^{ik_{\mathrm{e}}z} \rangle \\
&= c_1 \langle e^{-\alpha_1(x^2+y^2+z^2)} | e^{ik_{\mathrm{e}}z} \rangle + c_2 \langle e^{-\alpha_2(x^2+y^2+z^2)} | e^{ik_{\mathrm{e}}z} \rangle \\
&= c_1 \int_{-\infty}^{\infty} e^{-\alpha_1 x^2} \mathrm{d}x \int_{-\infty}^{\infty} e^{-\alpha_1 y^2} \mathrm{d}y \int_{-\infty}^{\infty} e^{-\alpha_1 z^2 + ik_{\mathrm{e}}z} \mathrm{d}z + \\
&+ c_2 \int_{-\infty}^{\infty} e^{-\alpha_2 x^2} \mathrm{d}x \int_{-\infty}^{\infty} e^{-\alpha_2 y^2} \mathrm{d}y \int_{-\infty}^{\infty} e^{-\alpha_2 z^2 + ik_{\mathrm{e}}z} \mathrm{d}z + \\
&= c_1 \left(\frac{\pi}{\alpha_1}\right)^{3/2} e^{-k_{\mathrm{e}}^2/(4\alpha_1)} + c_2 \left(\frac{\pi}{\alpha_2}\right)^{3/2} e^{-k_{\mathrm{e}}^2/(4\alpha_2)},
\end{aligned} \tag{S40}$$

where the integrals over $x$ and $y$ are each equal to $\sqrt{\pi/\alpha}$ and the integrals over $z$ have been evaluated using Eq. (S32).

The dipole photoionization cross-section will present a discontinuity for a $k_e$ that is a zero of the last expression in Eq. (S40), i.e. when:

$$c_1 \left(\frac{\pi}{\alpha_1}\right)^{3/2} e^{-k_{\mathrm{e}}^2/(4\alpha_1)} + c_2 \left(\frac{\pi}{\alpha_2}\right)^{3/2} e^{-k_{\mathrm{e}}^2/(4\alpha_2)} = 0. \tag{S41}$$

The above equation has two real solutions, one of which is positive:

$$k_e = \sqrt{\frac{4\alpha_1\alpha_2}{\alpha_2 - \alpha_1} \ln\left(-\frac{c_1 \alpha_2^{3/2}}{c_2 \alpha_1^{3/2}}\right)}, \tag{S42}$$

giving rise to a discontinuity at the corresponding photon energy.

In the case of Slater type orbitals (STOs), it can be shown that the transition matrix element has no zeros. To demonstrate this, we consider a 2s STO and a photoelectron described by a PW with wave-vector parallel to the z-axis, as in the previous case. The initial state is now:

$$\chi_{\mathrm{STO}} = r e^{-\xi r} \cos\theta, \tag{S43}$$

where the normalization constant has been left out for simplicity.

The transition matrix element to be calculated (in spherical coordinates, with volume element $r^2 \sin\theta \, \mathrm{d}r \, \mathrm{d}\theta \, \mathrm{d}\varphi$) is:

$$\begin{aligned}
\langle \chi_{\mathrm{STO}} | \chi_f \rangle &= \langle r e^{-\xi r} \cos\theta | e^{i k_\mathrm{e} r \cos\theta} \rangle \\
&= \int_0^{2\pi} \int_0^{\pi} \int_0^{\infty} r e^{-\xi r + i k_\mathrm{e} r \cos\theta} \cos\theta \; r^2 \sin\theta \, \mathrm{d}r \, \mathrm{d}\theta \, \mathrm{d}\varphi \\
&= 2\pi \int_0^{\pi} \frac{6 \sin\theta \cos\theta}{(\xi - i k_\mathrm{e} \cos\theta)^4} \, \mathrm{d}\theta = 32\pi \frac{i \xi k_\mathrm{e}}{(\xi^2 + k_\mathrm{e}^2)^3},
\end{aligned} \tag{S44}$$

which is zero only for $k_\mathrm{e} = 0$.

## REFERENCES

[1] J. Olsen and P. Jørgensen, J. Chem. Phys. **82**, 3235 (1985).

[2] D. N. Zubarev, *Nonequilibrium Statistical Thermodynamics* (Plenum Publishing Corporation, 1974).

[3] T. Petersson and B. Hellsing, Eur. J. Phys. **31**, 37 (2009).

[4] W. O. Straub, *A Brief Look at Gaussian Integrals* (Tech. Rep., 2009).
